# Supplementary material for: Your MMM is Broken: Identification of Nonlinear and Time-varying Effects in Marketing Mix Models
Source: arXiv:2408.07678 source file (2024-08-14)
Supplement: Supplementary file 1 [file illustration_parent.tex]

Here we provide an illustration for Remark \ref{interrelated}. We generated a ``common parent'' variable $\xi_t$ as a cosine function of time (Figure \ref{fig:commonp_xi}). Next, we generated $\beta_t$ as a GP over $\xi_t$  and $x_t$ as two invertible (log and square limited to the positive domain) and two non-invertible (square and cosine) functions of $\xi_t$. The response variable was generated under time-varying DGP:

\begin{equation*}
    y_t = a_0 + \beta_t x_t + \varepsilon_t
\end{equation*}

\begin{figure}[h]
    \centering
    \caption{Common parent: $\xi_t$ over time}
    \includegraphics[width = 0.7\textwidth]{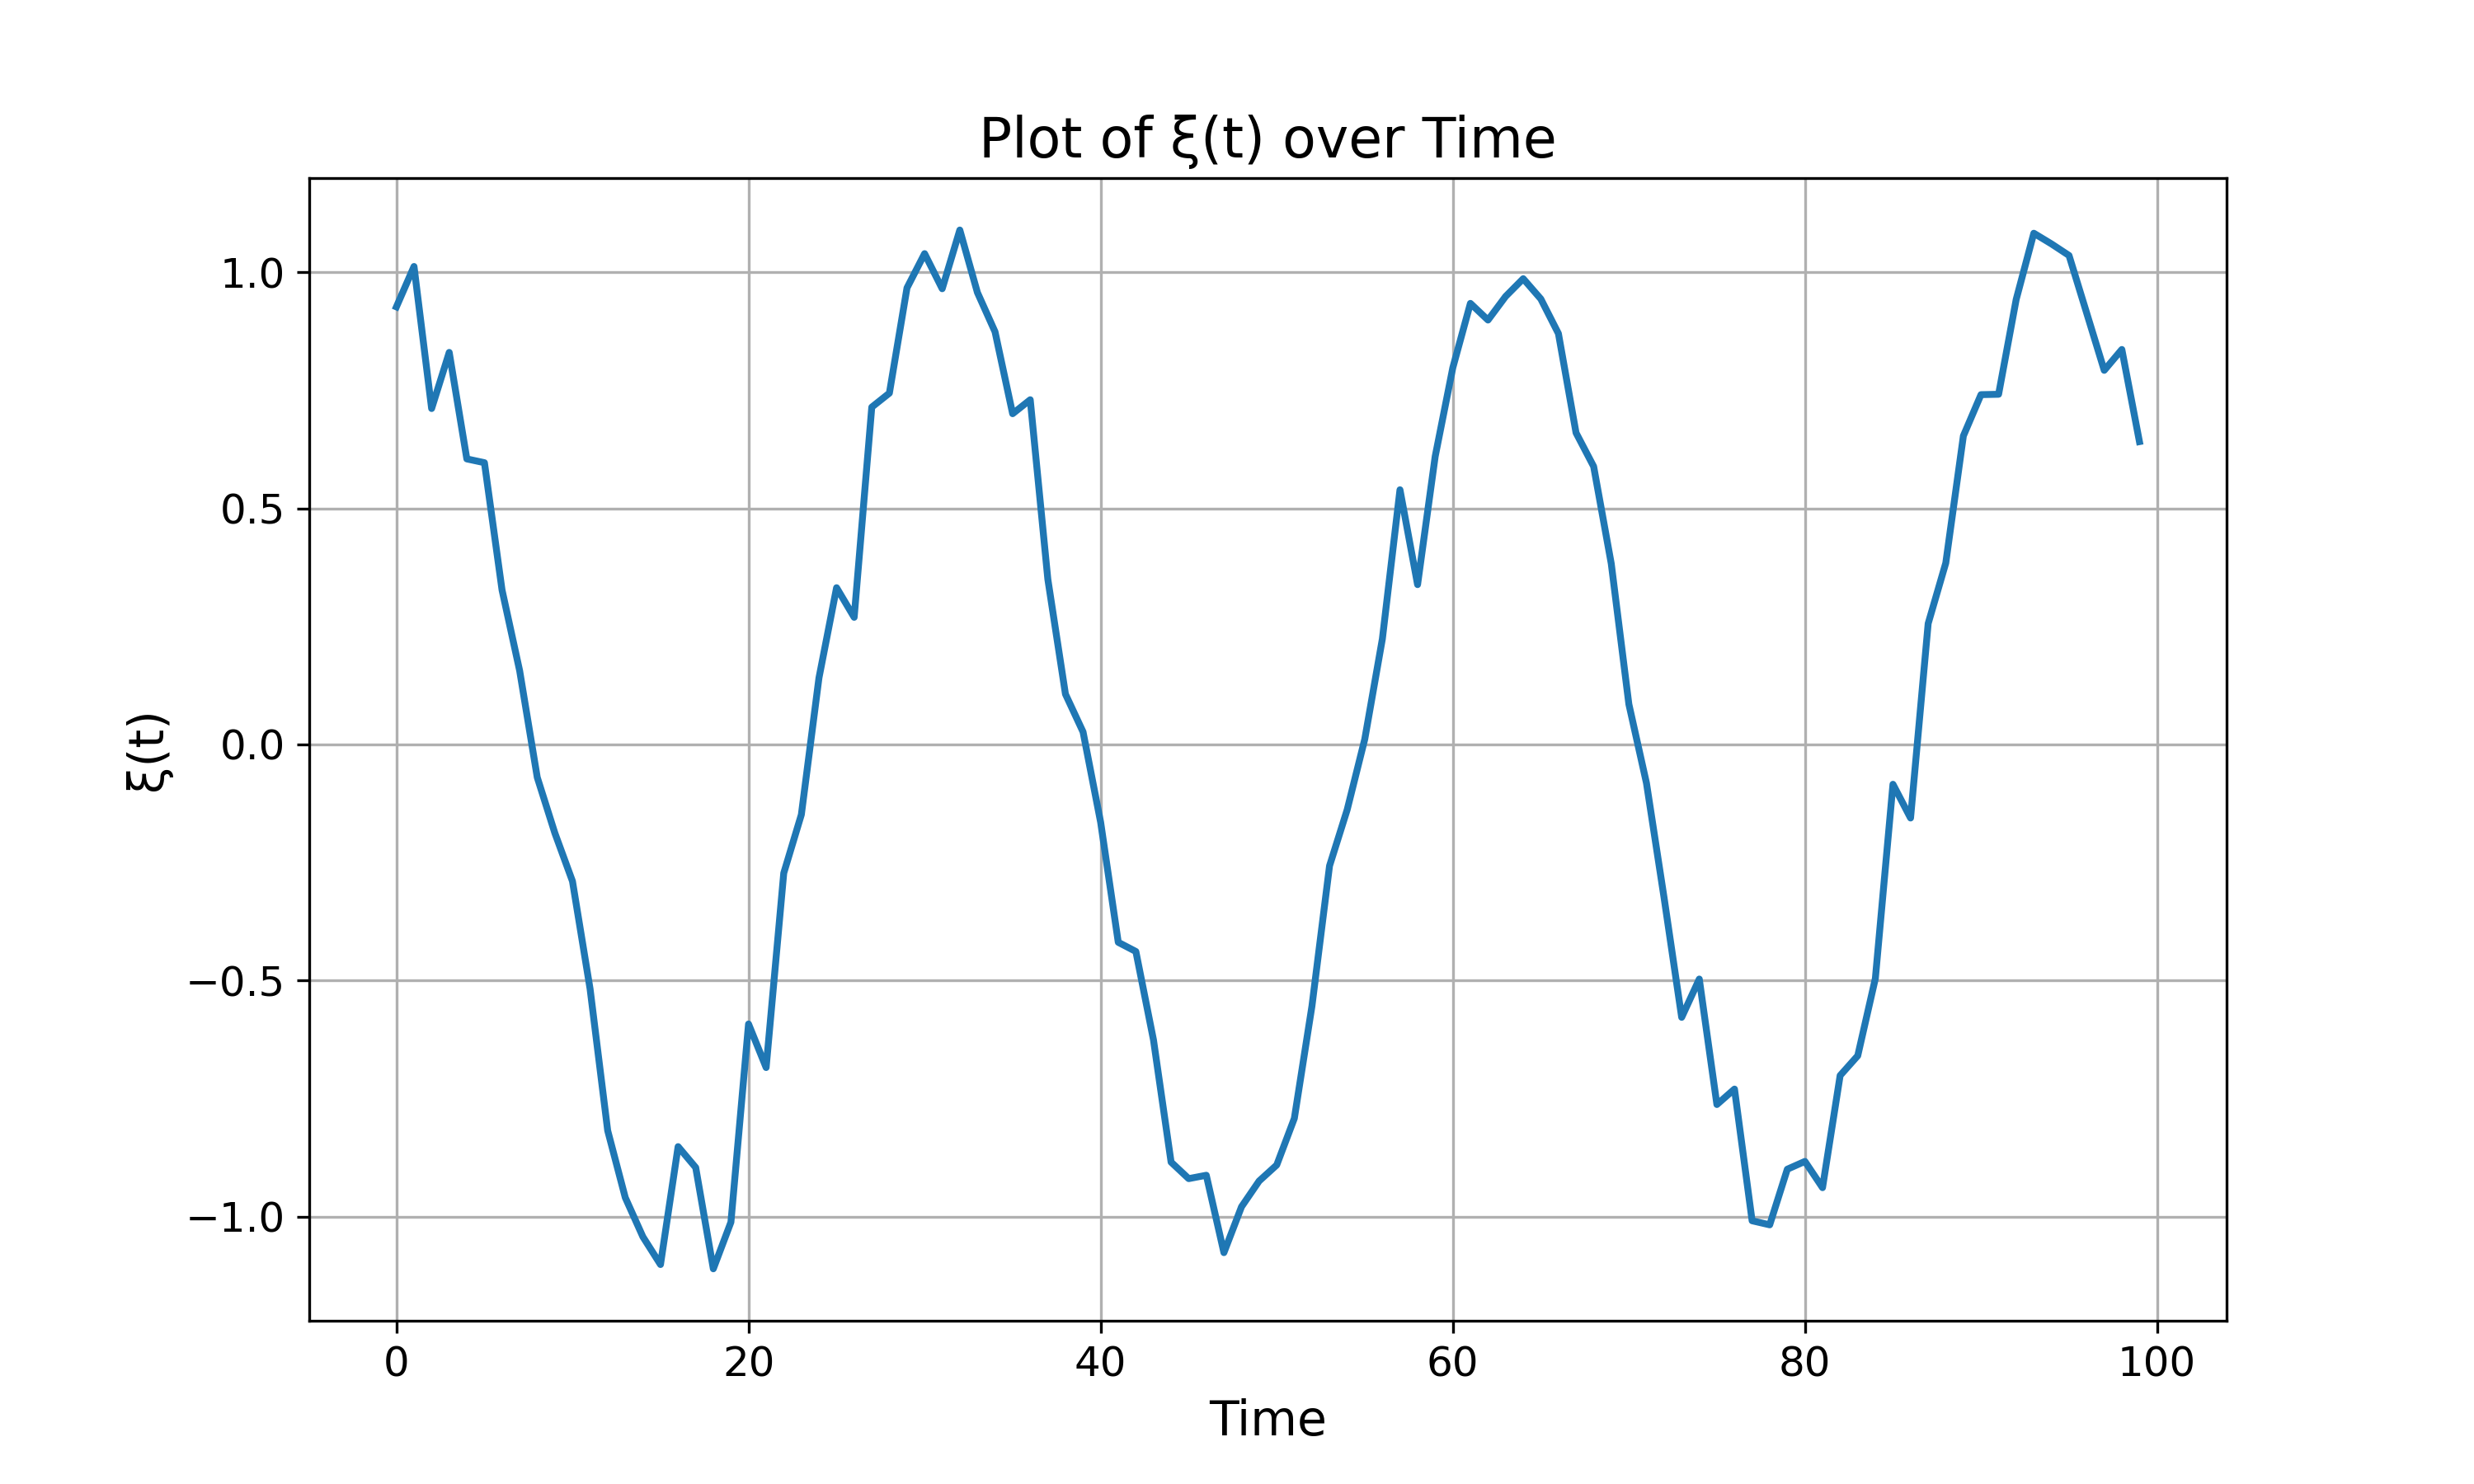}
    \label{fig:commonp_xi}
\end{figure}

\begin{figure}[h]
    \centering
    \caption{Common parent: $\beta_t$ is a GP over $\xi_t$}
    \includegraphics[width = 0.7\textwidth]{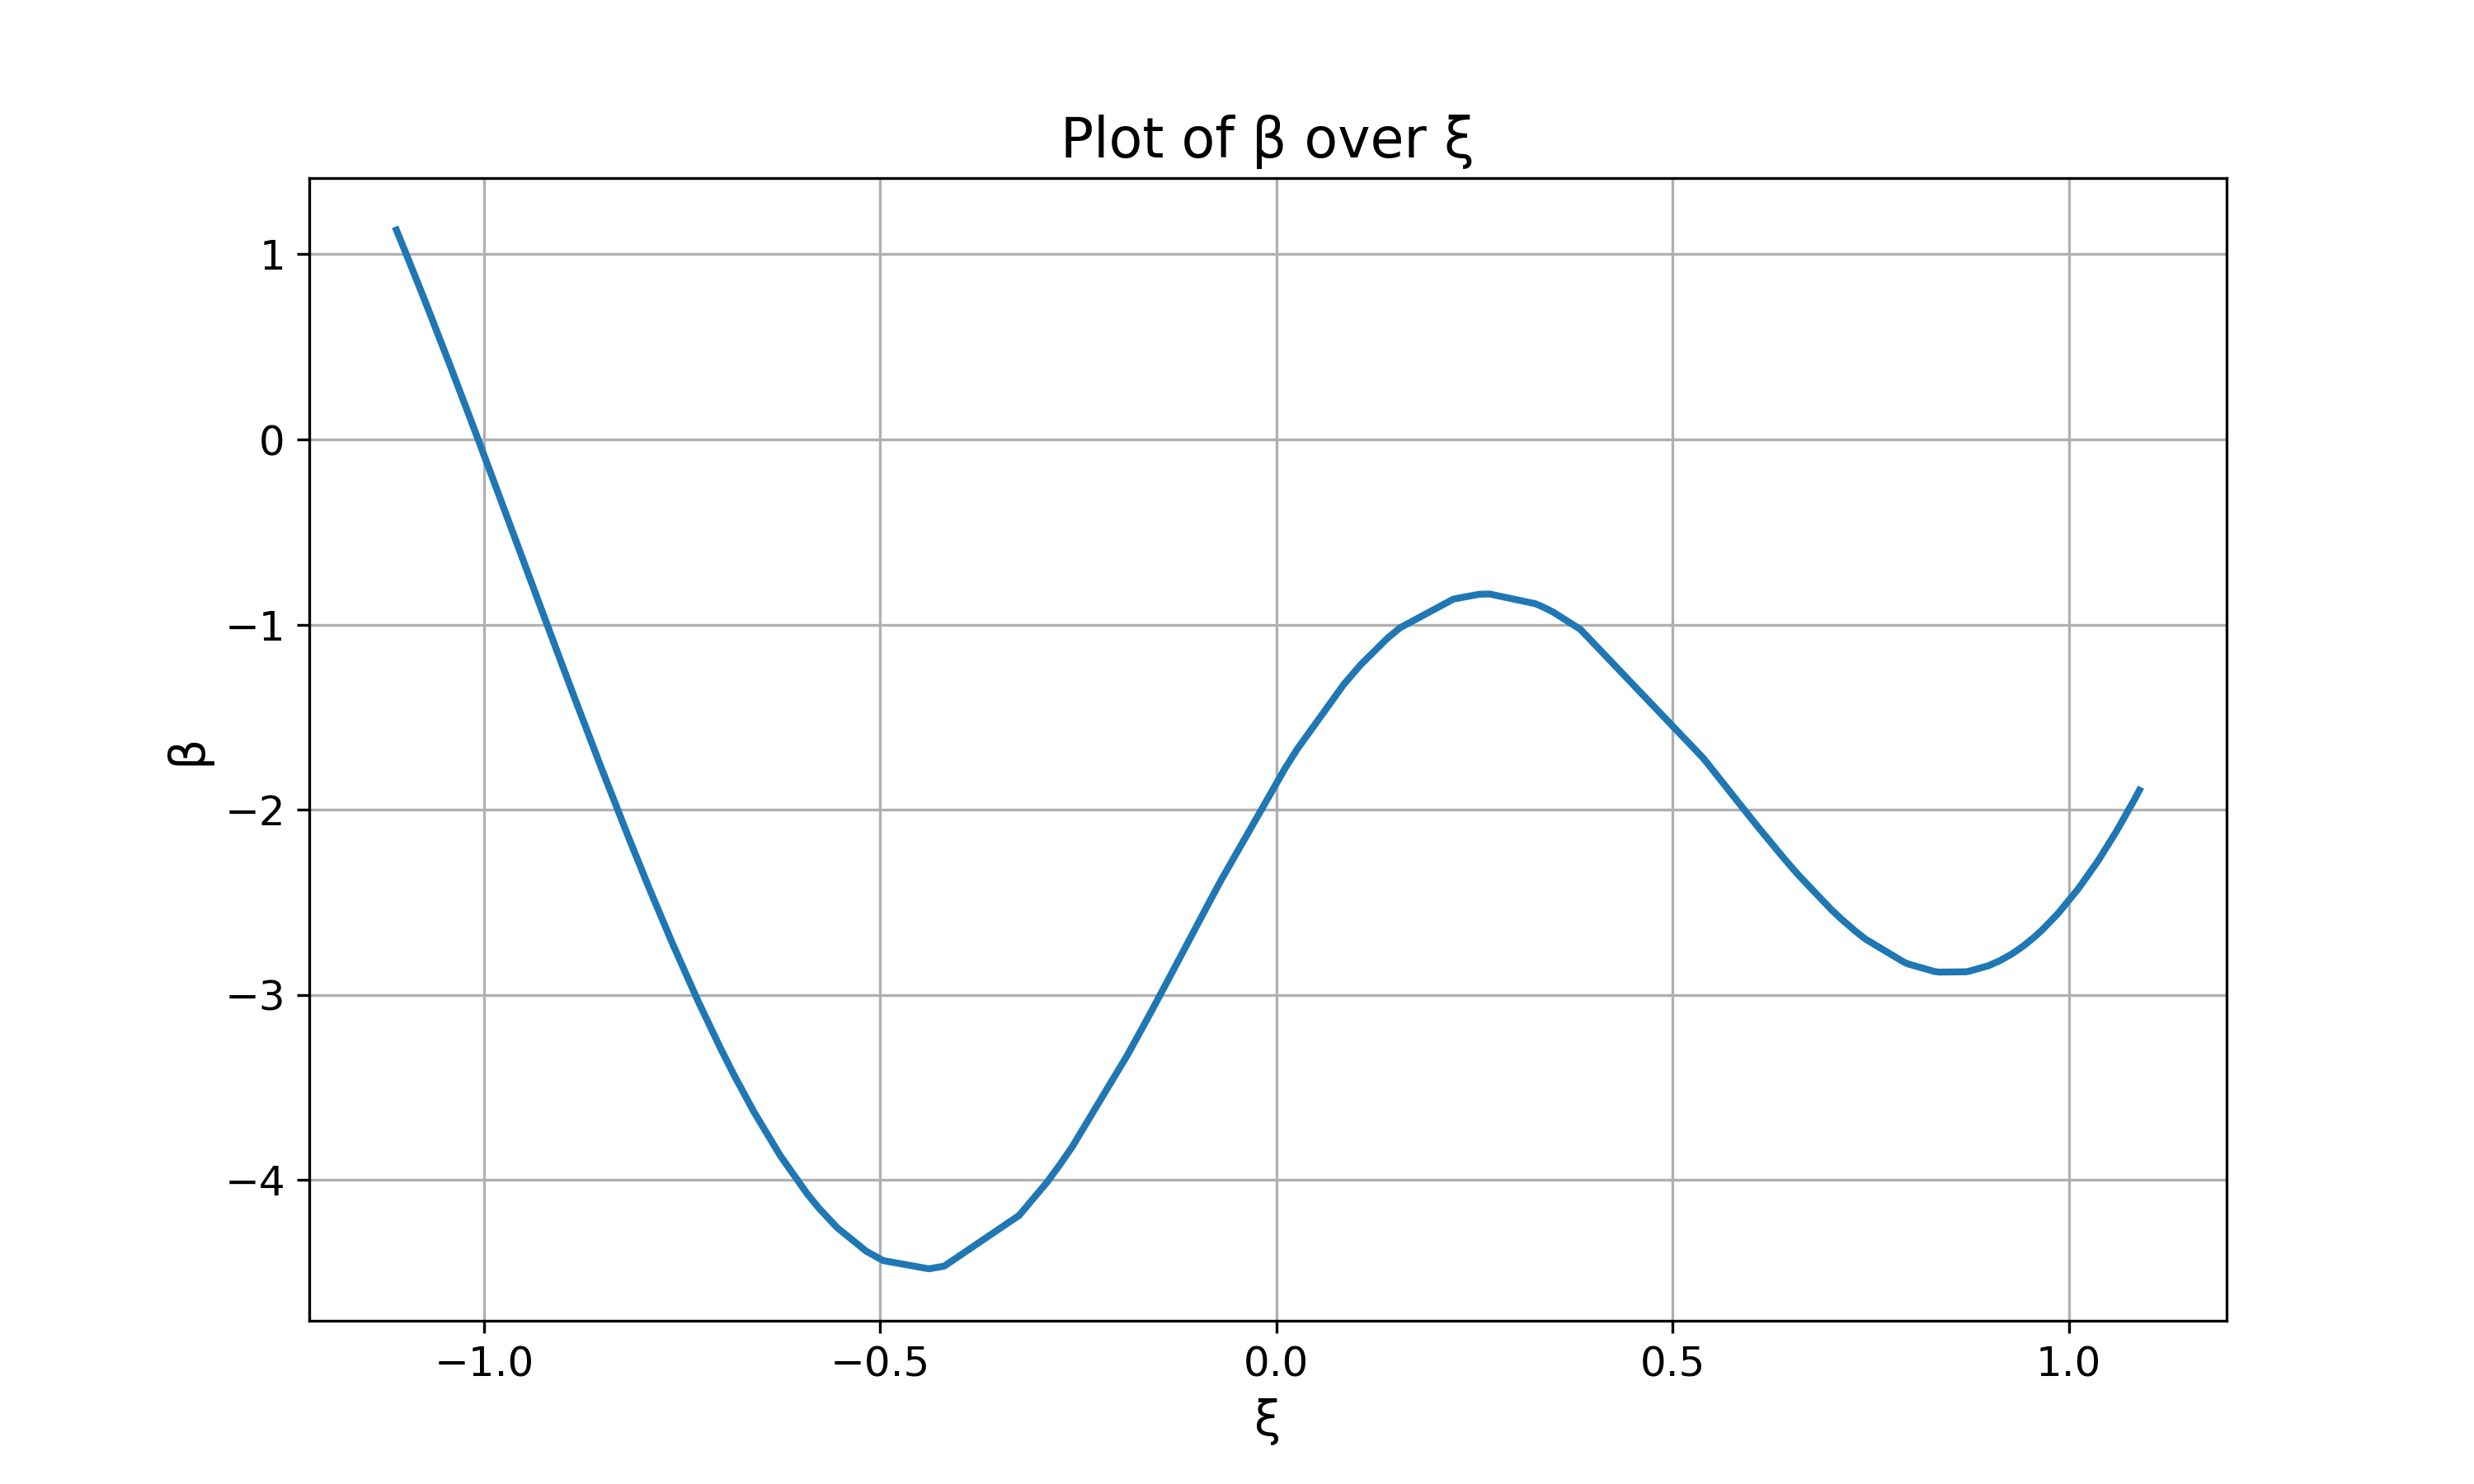}
    \label{fig:commonp_betaxi}
\end{figure}

\begin{figure}[h]
    \centering
    \caption{Common parent: $\beta_t$ over time}
    \includegraphics[width = 0.7\textwidth]{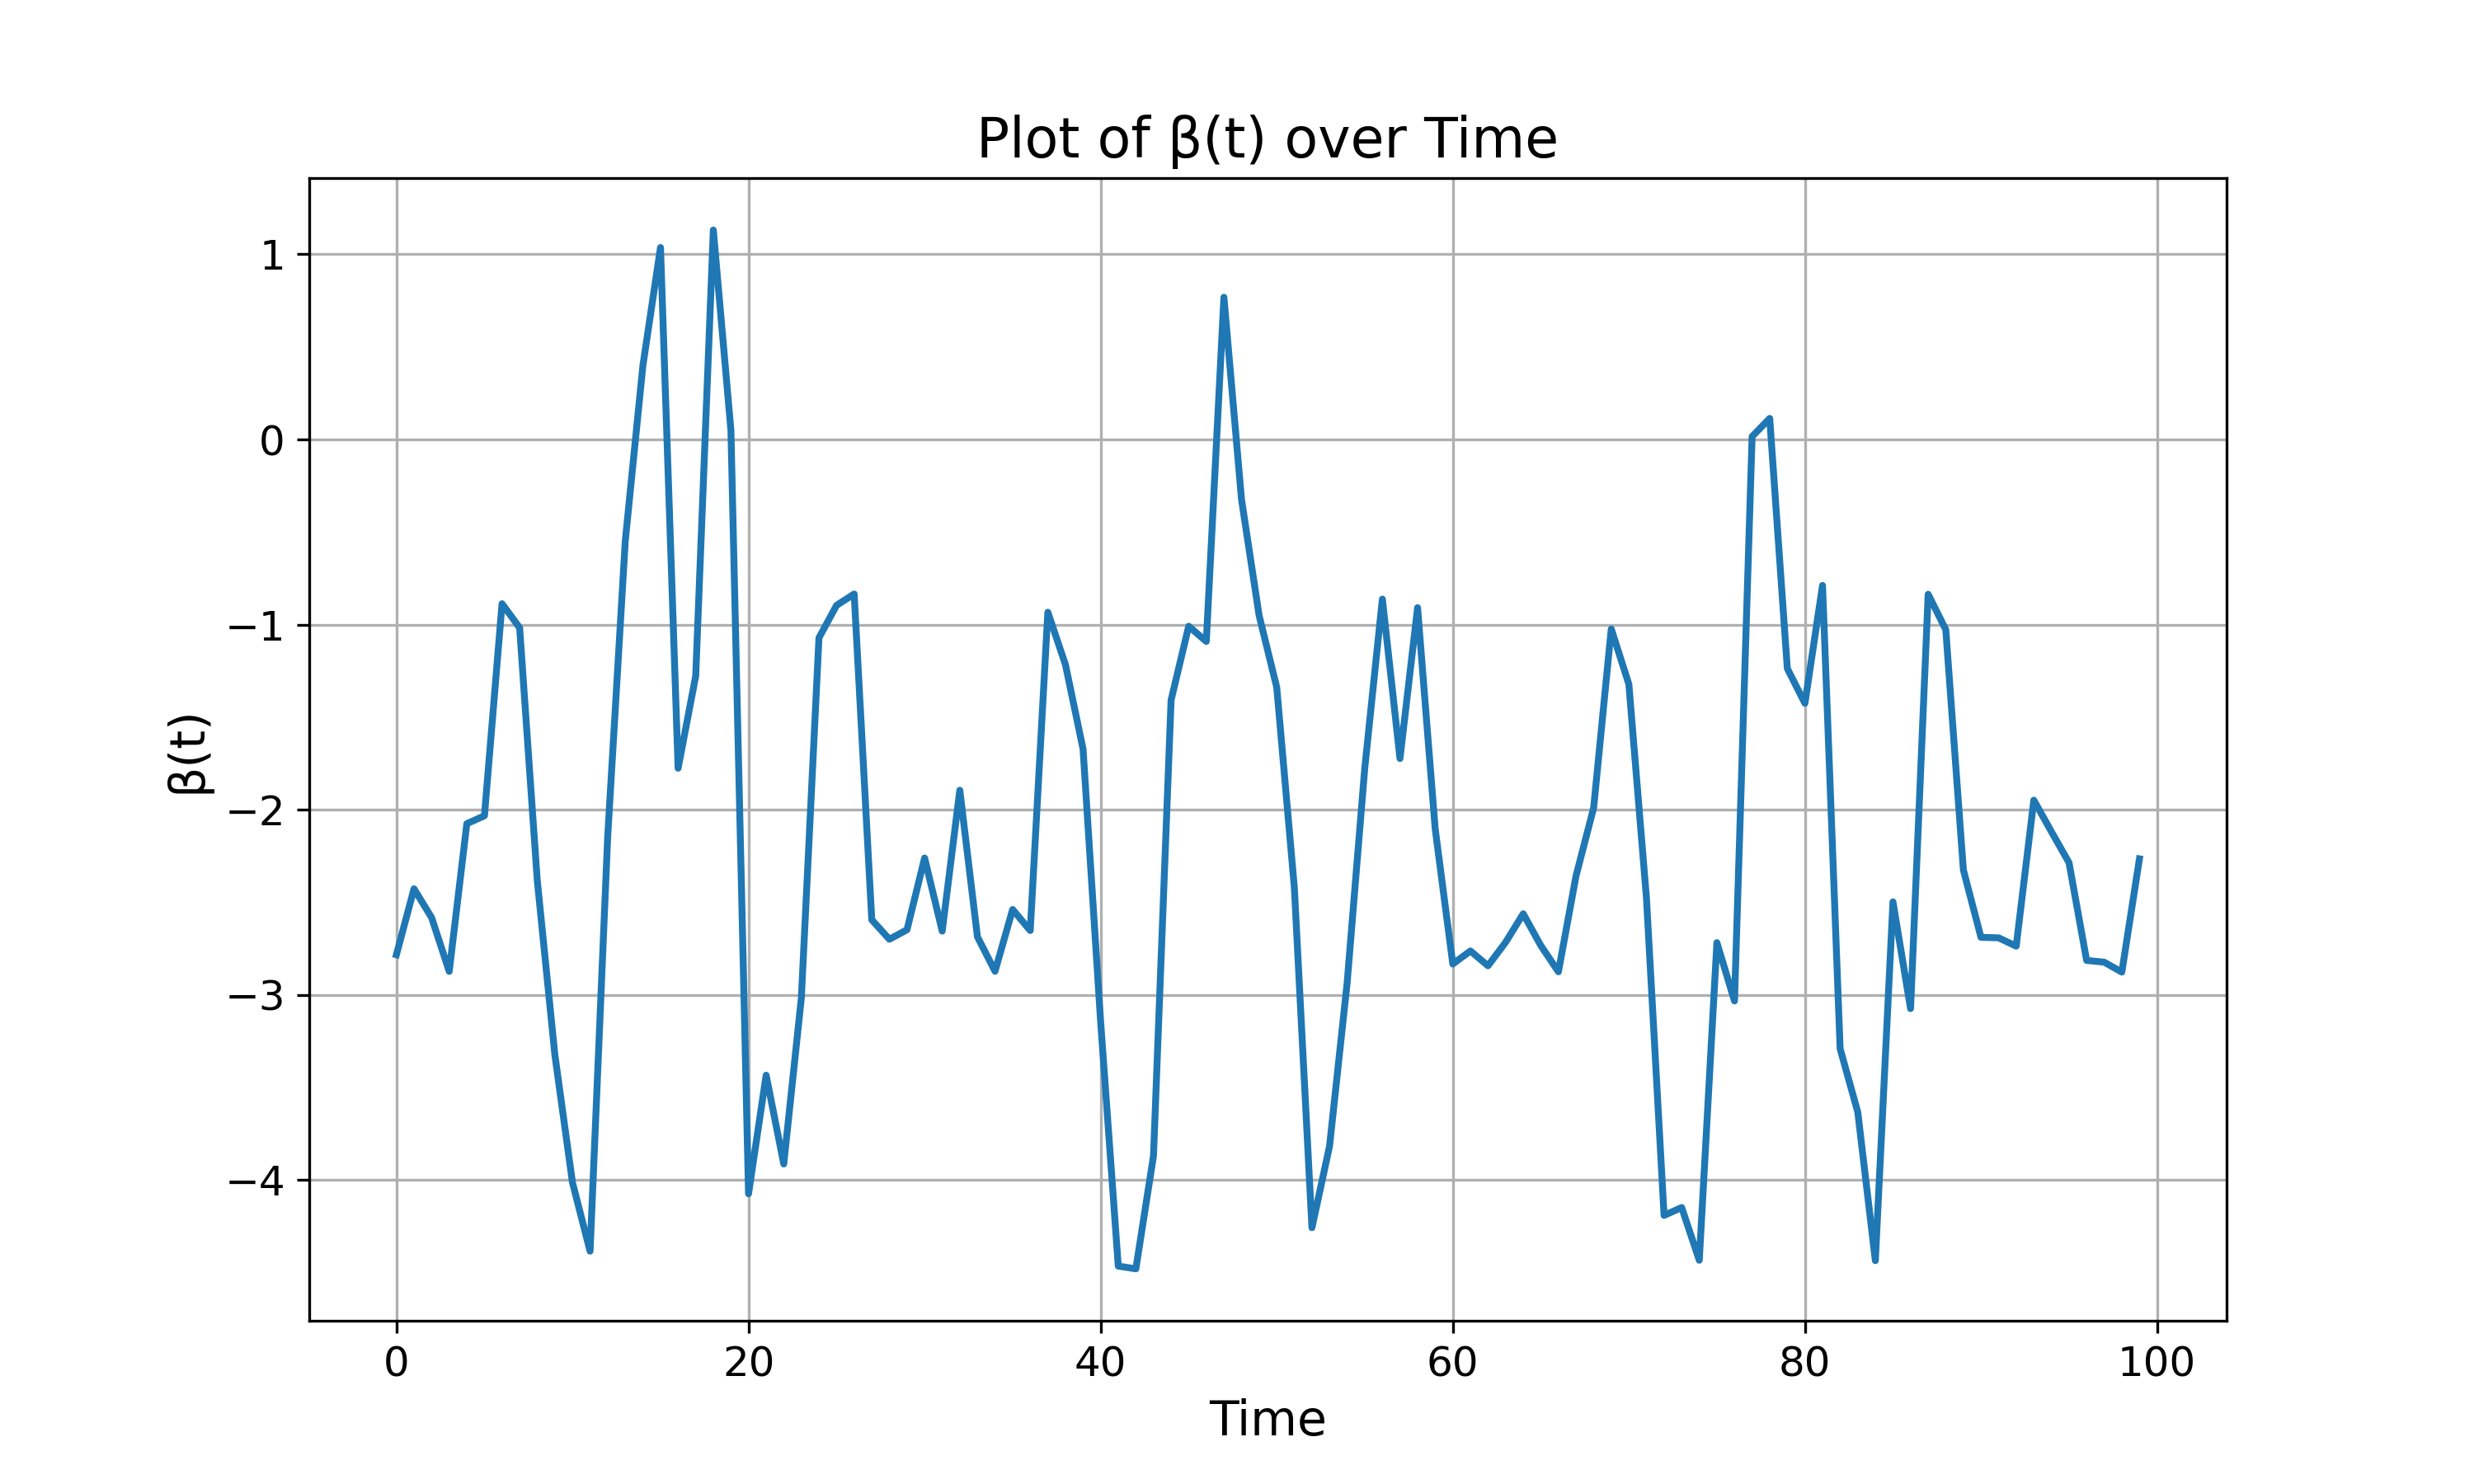}
    \label{fig:commonp_betatime}
\end{figure}

We estimate a static nonlinear GP model and a linear model with time-varying GP coefficients for each of the four functional forms of $x_t$. Figure \ref{fig:commonp_res} presents the results. As stated in Remark \ref{interrelated}, for the top two rows (corresponding to invertible functions of $x_t$ over $\xi_t$), the DGP can be fully expressed as a static non-linear DGP, which is picked up by the static nonlinear Gaussian Process model and results in a lower MSE on a holdout sample compared to the time-varying GP model, representing the true underlying DGP.

\begin{figure}[htbp]
    \centering
    \caption{Common parent: Invertible vs non-invertible $x(\xi_t)$}
    \includegraphics[width = \textwidth]{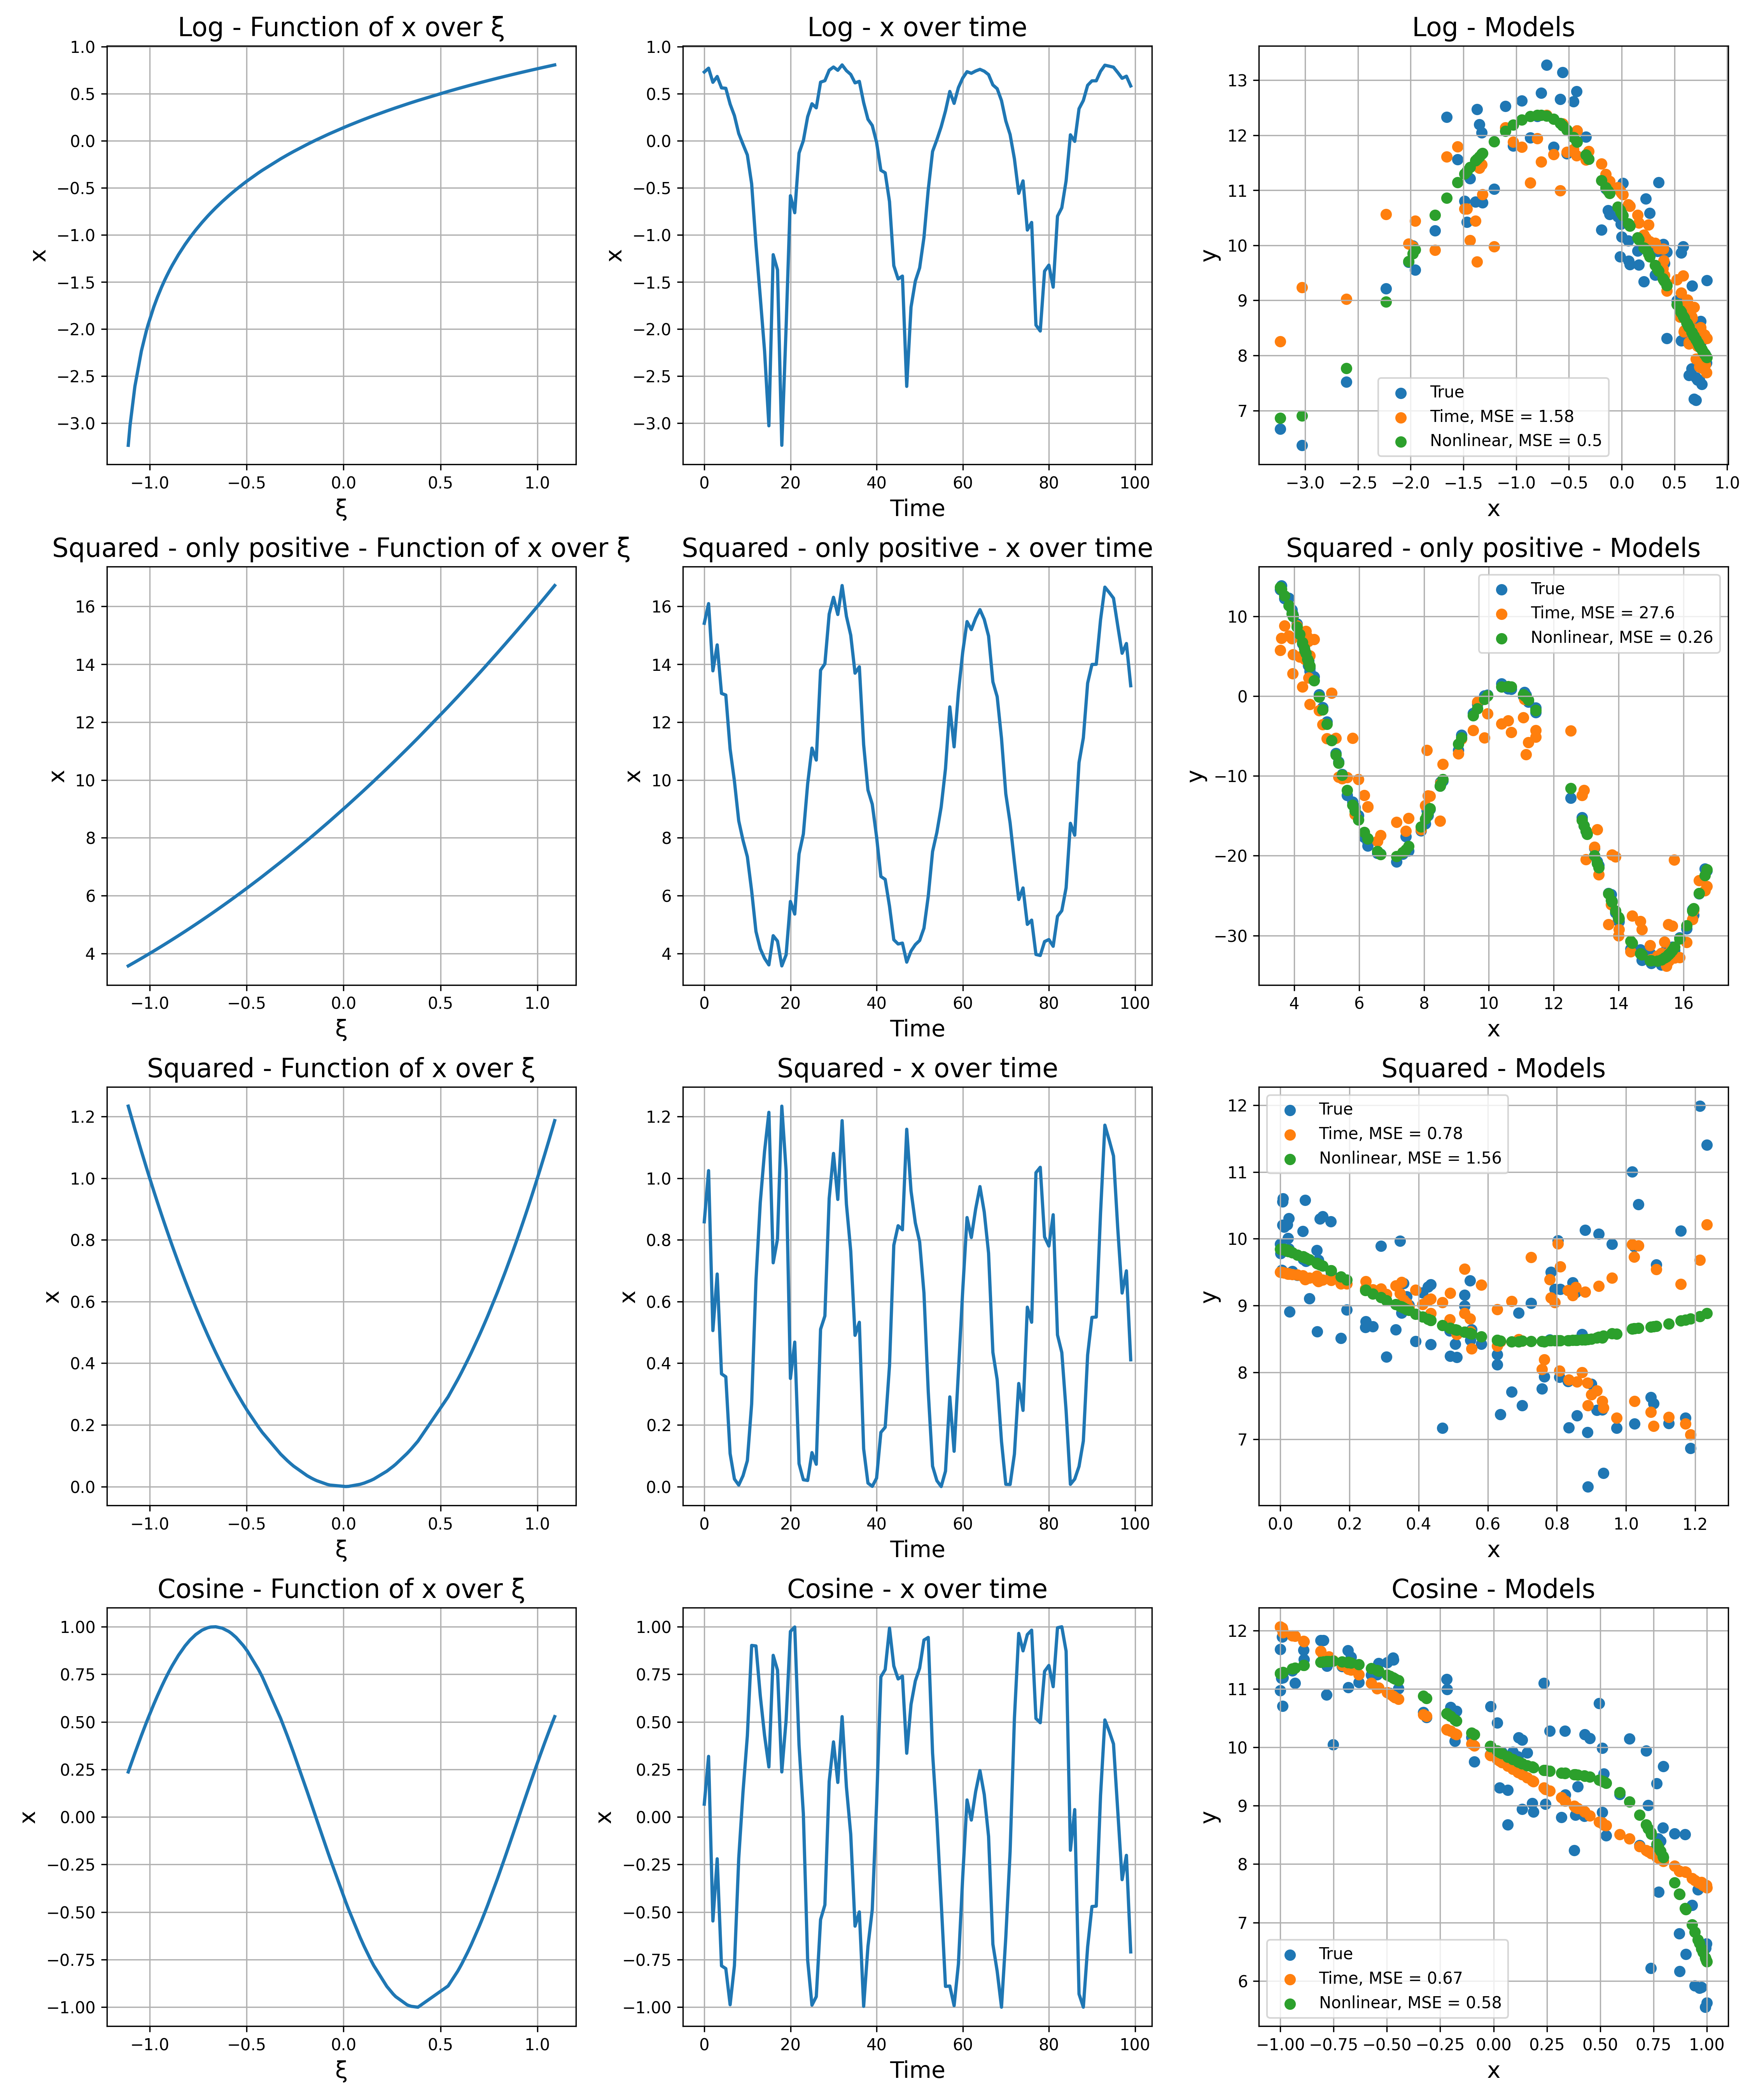}
    \label{fig:commonp_res}
\end{figure}

In the bottom two rows, the funciton of $x_t$ over $\xi_t$ is no longer monotone, and thus $y_t$ over $x_t$ is not guaranteed to have a representation as a static nonlinear DGP. Row 3 ($x_t$ is a squared function of $\xi_t$) provides an illustration. For $x_t \ge 0.6$, $y_t$ ``splits'' into two separate functions. The time-varying GP model is able to accurately capture this pattern, while the nonlinear GP model can only predict the mean of the ``split''. As a result, the time-varying GP model has a lower MSE.

The last row, however, illustrates, that invertibility of $x_t$ as a function of $\xi_t$ is not a necessary condition for $y_t$ over $x_t$ to be adequately captured by a static nonlinear DGP. Even though $x_t$ is a nonmonotone cosine function of $x_t$, $y_t$ over $x_t$ still looks nonlinear, and the static GP model provides a lower MSE compared to the time-varying GP model.
