# Supplementary material for: Your MMM is Broken: Identification of Nonlinear and Time-varying Effects in Marketing Mix Models
Source: arXiv:2408.07678 source file (2024-08-14)
Supplement: Supplementary file 2 [file math.tex]

\documentclass{article}
\usepackage{graphicx} % Requimagenta for inserting images
\input{preamble}

\title{Identification of Nonlinear and Dynamic Effects in Marketing Mix Models}
\author{Ryan Dew, Nicolas Padilla, Anya Shchetkina}
\date{November 2023}

\begin{document}

\maketitle

\section{Measurement frameworks}

\subsection{Mathematical illustration}

\subsubsection{Assumptions on the data generating process}

We assume outcomes are a nonlinear function of the input plus iid noise

\begin{assumption}[DGP]\label{dgp}
\[y_i = f(x_i)+\varepsilon_i, \quad  \varepsilon_i\sim\N(0,\sigma^2).\]
\end{assumption}

We state explicitly the relationship of $x_i$ and $\varepsilon_i$, which will be useful when assessing the convergence of the OLS estimator.

\begin{remark}[Uncorrelated errors]\label{uncorrelated}
  $\E(\varepsilon_i\cdot x_i)=0$ (directly from the dgp).
\end{remark}

We require $f$ to be differentiable for the Taylor expansion. 
%We also require observations to be iid in order to use $\xbar\convd E(x)$. 
%We need to extend these calculations later for the time-series models (i.e., random walk and AR(1)). Finally, we need an assumption that describes what ``$x$ very closely around the mean'' actually means. 

\begin{assumption}[Differentiable]\label{cond_diff}
  $f$ is differentiable up to order $K>2$.
\end{assumption}

% \begin{assumption}[iid]\label{iid}
%   $\lbrace x_i\rbrace^n_{i=1}$ are i.i.d.
% \end{assumption}

% \begin{assumption}[Around the mean]\label{around_mean}
%   {\color{magenta} {\tt This is one of the assumptions we need to tweak}}
%   $$\frac{\E\left[(x-\E(x))^3\cdot f''(x)\right]}{\E\left[(x-\E(x))^2\right]}\approx 0$$ 
% \end{assumption}

Under Assumption~\ref{cond_diff} we can write $f$ using its Taylor expansion of degree 1 around $\xbar=\frac{1}{n}\sum^n_{i=1}x_i$, 
\begin{align}
    f(x) &= f(\xbar) + f'(\xbar)(x-\xbar)+R_1(x) \label{eq:taylor}
\end{align}
where 
\begin{align*}
    R_1(x) &= \frac{f''(\xi)}{2}(x-\xbar)^2 & (\text{Lagrange form})\\
    &= \int\limits^x_{\xbar}\frac{f''(t)}{1!}(x-t) dt & (\text{Integral form})
\end{align*}
 with $\xi$ between $x$ and $\xbar$.

\subsubsection{Local linear regression}
Consider the linear (approximation) model
\begin{equation}
y_i=b_0+b_1x_i+\epsilon_i,
\end{equation}
and the corresponding OLS estimator 
\begin{align}
    \hat{b}_1 &= \frac{\sum_i(x_i-\bar{x})(y_i-\bar{y})}{\sum_i(x_i-\bar{x})^2}\label{eq:b1_hat}\\
    \hat{b}_0 &= \bar{y}-\hat{b}_1\bar{x}\nonumber
\end{align}
Note that by definition
\begin{equation}
\epsilon_i=y_i-(b_0+b_1x_i)=\left[f(x_i)-(b_0+b_1x_i)\right]+\varepsilon_i.
\end{equation}
% We start be writing $\bar{y}$ using the Taylor expression in \eqref{eq:taylor},
% \begin{align*}
%     \bar{y} &= \frac{1}{n}\sum_j y_j\\
%     &= \frac{1}{n}\sum_j \left[f(x_j)+\varepsilon_j\right]\\
%     &= \frac{1}{n}\sum_j \left[f(\xbar)+f'(\xbar)(x_j-\xbar)+\frac{1}{2}f''(\xbar)(x_j-\xbar)^2+R_2(x_j) \right]+\bar{\varepsilon}\\
%     &= \frac{1}{n}\sum_j \left[f'(\xbar)(x_j-\xbar)+\frac{1}{2}f''(\xbar)(x_j-\xbar)^2+R_2(x_j) \right]+f(\xbar)+\bar{\varepsilon}
% \end{align*}

We can rewrite \eqref{eq:b1_hat} as well using \eqref{eq:taylor}

\begin{align}
    \sum_i(x_i-\bar{x})(y_i-\bar{y}) &= \sum_i(x_i-\bar{x})\left[f(x_i)+\varepsilon_i-\bar{y}\right]\nonumber\\
    &= \sum_i(x_i-\bar{x})\left[f(x_i)+\varepsilon_i\right]-\bar{y}\sum_i(x_i-\bar{x})\nonumber\\
    &= \sum_i(x_i-\bar{x})\left[f(x_i)+\varepsilon_i\right]\nonumber\\
    &= \sum_i(x_i-\bar{x})\left[f(\xbar)+f'(\xbar)(x_i-\xbar)+R_1(x_i)+\varepsilon_i\right]\nonumber\\
    &= \sum_i(x_i-\bar{x})\left[f'(\xbar)(x_i-\xbar)+R_1(x_i)+\varepsilon_i\right]\nonumber\\
    &= f'(\xbar)\sum_i(x_i-\bar{x})^2+\sum_i(x_i-\xbar)R_1(x_i)+\sum_i(x_i-\xbar)\varepsilon_i\nonumber\\
    &= f'(\xbar)\sum_i(x_i-\bar{x})^2+\frac{1}{2}\sum_if''(\xi_i)(x_i-\xbar)^3+\sum_i(x_i-\xbar)\varepsilon_i\label{numerator}
\end{align}
Now replacing \eqref{numerator} in \eqref{eq:b1_hat}, we have

\begin{align}
    \hat{b}_1 &= \frac{1}{\sum_i(x_i-\bar{x})^2}\left[ f'(\xbar)\sum_i(x_i-\bar{x})^2+\frac{1}{2}\sum_if''(\xi_i)(x_i-\xbar)^3+\sum_i(x_i-\xbar)\varepsilon_i\right]\nonumber\\
    &=  f'(\xbar)+\frac{1}{2}\frac{\frac{1}{n} \sum_if''(\xi_i)(x_i-\xbar)^3}{\frac{1}{n} \sum_i(x_i-\bar{x})^2}+\frac{\frac{1}{n} \sum_i(x_i-\xbar)\varepsilon_i}{\frac{1}{n} \sum_i(x_i-\bar{x})^2}\label{eq:b1_hat_as_fn_of_f}
\end{align}

\subsection{Time series}

% By Assumption\ref{iid}, we get $\xbar\convp E(x)$. Using the Continuous Mapping Theorem, 
% \begin{equation}
% f'(\xbar)\convp f'(\E(x)).
% \end{equation}

% By (weak) LLN, 
% \begin{align}
% \frac{1}{n} \sum_i(x_i-\xbar)\varepsilon_i&\convp \E((x-\E(x))\varepsilon)=0\\
% \frac{1}{n} \sum_i(x_i-\xbar)^2&\convp \E((x-\E(x)^2)
% \end{align}

% {\color{magenta}I am not sure exactly what assumptions we need, but I assume some form of squeeze condition on $f''(\xi_i)$. 

% For example, we could assume that the derivative is bounded or reaches a maximum $\vert f''(\xi_i)\vert \leq \lambda,\; \forall x \in B$ (which we can get with $x$ leaving in a closed interval, and $f$ begin continuous). That would allow us to approximate 
% }

% By LLN, 
% \begin{align}
% \frac{1}{n} \sum_if''(\xi_i)(x_i-\xbar)^3&\convp \E\left[f''(x)(x-\E(x))^3\right]
% \end{align}

% Using Assumption \ref{around_mean}, we have that 
% $$\hat{b}_1\convp f'(\E(x))+\frac{\E\left[(x-\E(x))^3\cdot f''(x)\right]}{\E\left[(x-\E(x))^2\right]}\approx f'(\E(x))$$

\section*{Appendix: Other calculations}

\subsection*{Random walk}

{
    \color{magenta} My intuition is that we need a Brownian motion instead. This is because we can set a continuous interval around $t$, and then center the analysis on $x(t)$, for example, looking at the interval $[t-\Delta,t+\Delta]$. Then, we can sample $n$ observations, $t_1,\ldots,t_n$ in $[t-\Delta,t+\Delta]$, and define $\widetilde{x}_i = x(t_i)$. If $t_i$ are iid, that implies $\widetilde{x}_i$ are also iid, and we can use the results derived above. We can use the same approach for the AR(1).
}
\begin{figure}[H]
    \centering
    \begin{tikzpicture}
      \begin{axis}[ 
        xlabel=$t$,
        ylabel={$x$},
        xtick=\empty, 
        ytick=\empty,
        ymin=-0.5,
      ] 
      \def\clippath{
        (-1.5,-0.5) rectangle (1.5,1.5)
        }
        \draw [help lines, dashed] \clippath;
        \addplot[
            smooth
        ] {1/(exp(-(x+1))+1)}; 
        \addplot[
            smooth, 
            domain=-1.5:1.5,
            blue
            ] 
        {(exp(-1)/(1+exp(-1))^2)*x+1/(1+exp(-1))}; 
        \addplot coordinates {
        (0,-0.5) (0,0.731058)
        } node [pos=1, yshift=15pt] {$x(t)$} ;
        \addplot[only marks] coordinates {
        (-1.5,-0.49) (1.5,-0.49)
        } [every node/.style={yshift=8pt}]
            node [pos=0, xshift=-15pt]  {$t-\Delta$}
            node [pos=1, xshift=15pt]  {$t+\Delta$}
        ;
      \end{axis}
    \end{tikzpicture}
    \caption{Local approximation}
    \label{fig:local_approx}
\end{figure}

\subsubsection*{Properties}

Starts at $x_0$ (known), and evolves according to $$x_{t} = x_{t-1} + e_{t}, \quad e_t\sim\N(0,\tau^2)$$

Let's compute its moments,
\begin{align}
    x_t &= x_0 + \sum^t_{s=1} e_s \\
    \implies \E(x_t) &= x_0 \\
    \implies \Var(x_t) &= \sum^t_{s=1} \Var(e_s) = t\cdot \tau^2\\
    \implies \E\left(\xbar(t)\right) &= \E\left(\xbar(t)\right) \\
\end{align}
What about the sample mean $\xbar(t)=\frac{1}{t}\sum^t_{s=1}x_s$?
\begin{align}
    \E\left(\xbar(t)\right) &= \frac{1}{t}\sum^t_{s=1} \E(x_s)=x_0
\end{align}

\end{document}
