# Supplementary material for: Your MMM is Broken: Identification of Nonlinear and Time-varying Effects in Marketing Mix Models
Source: arXiv:2408.07678 source file (2024-08-14)
Supplement: Supplementary file 3 [file sim_results_w_hill.tex]

\begin{table}[p]
\centering
\begin{tabular}{llrrrrrrrr}
\toprule
 & & \multicolumn{2}{c}{{Nonlinear DGP}} & &\multicolumn{2}{c}{{Dynamic DGP}} & &\multicolumn{2}{c}{{Hill DGP}} \\
\cmidrule(lr){3-4} \cmidrule(l){6-7} \cmidrule(l){9-10}
                {Variable} & {Level}  & {Coef} &  {$P(>\!|t|)$}    & & {Coef} & {$P(>\!|t|)$}  & & {Coef} & {$P(>\!|t|)$} \\
\midrule
Amplitude, $f$: & Low     & - & - & & - & - & & - & - \\
 & Middle & -0.06         & 0.94        &                  & 2.94          & 0.01  &  & - & -                     \\
&   High  & -0.11         & 0.88        &                  & 8.99          & 0.00  &  & - & -                     \\
\midrule
Smoothness, $f$: & Low & - & - & & - & - & & - & - \\
 & Middle & 9.99          & 0.00       &                   & 3.44          & 0.00        & & - & -               \\
 & High   & 19.43         & 0.00       &                   & 8.10          & 0.00        & & - & -               \\
 \midrule
 Infliction point, $f$: & Low & - & - & & - & - & & - & - \\
 & Middle & -         & -       &                   & -          & -             & & -2.15 & 0.21          \\
 & High   & -         & -       &    -              & -        & -              & & 2.27 & 0.19         \\
 \midrule
 Shape parameter, $f$: & Very Low & - & - & & - & - & & - & - \\
  & Low & -          & -       &                   & -          & -         & & -2.44 & 0.27             \\
 & Middle & -          & -       &                   & -          & -         & & -7.06 & 0.00              \\
 & High   & -         & -       &                   & -          & -        & & -12.14 & 0.00              \\
  & Very High   & -         & -       &                   & -          & -       & & -15.44 & 0.00               \\
 \midrule
AR coef, $x$: & Low & - & - & & - & - & & - & - \\ 
 & Middle            & 0.81          & 0.28        &                  & 1.05          & 0.36          & & -0.10 & 0.95            \\
& High            & 2.66          & 0.00          &                & 4.77          & 0.00      & & 24.22 & 0.00                 \\
\midrule
Variance, $x$: & Low  & - & - & & - & - & & - & -\\
& Middle         & -0.16         & 0.83           &               & 5.80          & 0.00   & & - & -                    \\
& High        & 0.07          & 0.92               &           & 11.66         & 0.00    & & - & -                   \\
\midrule
Noise, $y$ & Low & - & - & & - & - & & - & - \\
& Middle       & 7.60          & 0.00             &             & 6.69          & 0.00    & & 11.16 & 0.00                  \\
& High       & 14.81         & 0.00              &            & 20.25         & 0.00    & & 20.20 & 0.00                   \\
& Very High     & 24.02         & 0.00           &               & 40.19         & 0.00    & & 27.00 & 0.00                   \\
\bottomrule
\end{tabular}
\tcaption{Simulation Results}{DV = Percentage Conflation; Intercept omitted for clarity.}
\label{tab:sim_deep_dive}
\end{table}
