# Supplementary material for: Your MMM is Broken: Identification of Nonlinear and Time-varying Effects in Marketing Mix Models
Source: arXiv:2408.07678 source file (2024-08-14)
Supplement: Supplementary file 4 [file tikz_diagram_parent.tex]

\begin{figure}
    \centering
    \begin{tikzpicture}
    % Variables
    \node[const]   (t)   {$t$}; %
    \node[const, below=of t, xshift=-0.8cm]   (x)   {$x_t$}; %
    \node[const, below=of t, xshift=0.8cm]   (beta)   {$\beta_t$}; %

    % Edges
    \edge {t} {x};
    \edge {t} {beta};
    
    \end{tikzpicture}
    \hfill
    \begin{tikzpicture}
    % Variables
    \node[const]   (t)   {$t$}; %
    \node[const, below=of t, xshift=-0.8cm]   (x)   {$x_t$}; %
    \node[const, below=of t, xshift=0.8cm]   (beta)   {$\beta_t$}; %

    % Edges
    \edge {t} {x};
    \edge {t} {beta};
    \draw[->,blue] (x) to[out=45,in=135] (beta);
    
    \end{tikzpicture}
    \hfill
    \begin{tikzpicture}
    % Variables
    \node[const]   (t)   {$t$}; %
    \node[const, below=of t, xshift=-0.8cm]   (x)   {$x_t$}; %
    \node[const, below=of t, xshift=0.8cm]   (beta)   {$\beta_t$}; %

    % Edges
    \edge {t} {x};
    \edge {x} {t};
    \edge {t} {beta};
    \draw[->,blue] (x) to[out=45,in=135] (beta);
    
    \end{tikzpicture}\hfill
    \begin{tikzpicture}
    % Variables
    \node[const]   (t)   {$t$}; %
    \node[const, below=of t]   (xi)   {$\xi_t$}; %
    \node[const, below=of xi, xshift=-0.8cm]   (x)   {$x_t$}; %
    \node[const, below=of xi, xshift=0.8cm]   (beta)   {$\beta_t$}; %

    % Edges
    \edge {t} {xi};
    \edge {xi} {x};
    \edge {x} {xi};
    \edge {xi} {beta};
    \draw[->,blue] (x) to[out=45,in=135] (beta);
    
    \end{tikzpicture}
    \caption{Caption}
    \label{fig:enter-label}
\end{figure}
